# Supplementary material for: Integrating Emotional and Linguistic Models for Ethical Compliance in Large Language Models
Source: arXiv:2405.07076 source file (2024-05-14)
Supplement: Supplementary file 3 [file AppendixZ.tex]

\subsection*{Appendix C}

\begin{table}[ht]
\centering
\begin{footnotesize}
\begin{tabular}{@{}ll@{}}
\toprule
\textbf{Emotion} & \textbf{Linguistic Features} \\ \midrule
Despair, Sadness, Melancholy & Negative adjectives, dark imagery, passive constructions \\
Contentment, Happiness, Joy & Positive adjectives, vivid imagery, exclamations \\
Terror, Fear, Anxiety & Negative adjectives, rhetorical questions, passive constructions \\
Boldness, Courage, Heroism & Positive adjectives, hyperbole, active voice \\
Rage, Anger, Irritation & Negative adjectives, dark imagery, short sentences \\
Composure, Peace, Tranquility & Balanced structures, calm imagery, long sentences \\
Shock, Surprise, Startle & Exclamations, short sentences, sudden changes in tone \\
Expect., Prepared, Anticipation & Future tense, modal verbs, conditional phrases \\
Revulsion, Disgust, Distaste & Negative adjectives, imagery of unpleasant sensations \\
Appreciation, Respect, Admire & Positive adjectives, superlatives, respectful tone \\
Paranoia, Distrust, Suspicion & Negative adjectives, rhetorical questions, guarded tone \\
Confidence, Trust, Faith & Positive adjectives, affirmations, assured tone \\ \bottomrule
\end{tabular}
\end{footnotesize}
\vspace{.1in}
\caption{Linguistic Features by Emotion}
\label{tab:emotion_linguistics}
\end{table}
